# Supplementary material for: Streaming Real-Time Trajectory Prediction Using Endpoint-Aware Modeling
Source: arXiv:2603.01864 source file (2026-03-02)
Supplement: Supplementary file 1 [file _supplementary.tex]

\documentclass[10pt,twocolumn,letterpaper]{article}

\usepackage{wacv}              %

\input{_constants}
\input{_macros}

\definecolor{wacvblue}{rgb}{0.21,0.49,0.74}
\usepackage[pagebackref,breaklinks,colorlinks,allcolors=wacvblue]{hyperref}

\begin{document}

\title{Supplementary Material for \\ \paperTitle}

\author{\authorBlock}
\maketitle

\input{_sections/12_supplementary}

{
    \small
    \bibliographystyle{ieeenat_fullname}
    \bibliography{_sections/11_references}
}

\end{document}
